# Supplementary material for: Enhanced magnon spin current using the bosonic Klein paradox
Source: arXiv:2109.00865 source file (2022-02-08)
Supplement: Supplementary file 1 [file Supplement.pdf]

# Supplementary Material: Enhanced magnon spin current using the bosonic Klein paradox

J. S. Harms[1,*] H. Y. Yuan[1,†] and Rembert A. Duine[1,2]
[1]*Institute for Theoretical Physics, Utrecht University, 3584CC Utrecht, The Netherlands and*
[2]*Department of Applied Physics, Eindhoven University of Technology, P.O. Box 513, 5600 MB Eindhoven, The Netherlands*
(Dated: January 10, 2022)

In this supplementary material, we compare the original and magnon Klein paradox in detail, specify the parameters used in our micromagnetic simulations, and further clarify the correlations between incident, reflected and transmitted magnon spin currents.

## DETAILED COMPARISON BETWEEN ORIGINAL AND MAGNON KLEIN PARADOX

In this section, we address the analogue between the original Klein paradox and the magnon Klein paradox presented in the main text. In the original Klein paradox, Klein studied scattering of an electron off a potential barrier [1], as shown in the top panel of Fig. 1(a). The electrostatic potential in the right domain will lift the negative energy band of positrons [blue line in Fig. 1(a)] and makes it overlap with the positive energy band of electrons on the left (red line). Then, the incident electrons from the left domain can excite positron current moving to the right in the right domain. This corresponds to left-moving electron current and thus could enhance the reflection of electrons at the interface. A detailed treatment of this scattering process can be found in the literature [2]. In the magnon Klein paradox, an inhomogeneous external field, for example, can induce the band overlap of the magnons band in the left domain with the antimagnon band in the right domain, as shown in Fig. 1(b). Again, the antimagnon current generated at the interface enhances the strength of the reflected magnon current. The underlying physics of the original and magnon Klein paradox is therefore the same. This is so despite that the magnon bands on the left and right domains also overlap, but their coupling is very weak in our setup, and thus does not change the essential physics.

## PARAMETER SPECIFICATION IN NUMERICAL SIMULATIONS

The magnetization dynamics of the two exchange-coupled magnetic films are simulated by numerically solving the Landau-Lifhsitz-Gilbert (LLG) equations

$$\frac{\partial \mathbf{n}_\nu}{\partial t} = -\gamma \mathbf{n}_\nu \times \mathbf{h}_{\mathrm{eff},\nu} + \alpha \mathbf{n}_\nu \times \frac{\partial \mathbf{n}_\nu}{\partial t} + J_\nu \mathbf{n}_\nu \times \hat{z} \times \mathbf{n}_\nu, \tag{1}$$

where $\mathbf{n}_\nu$ is the normalized magnetization, $\nu = L, R$ labels the (L)eft and (R)ight magnet, $\gamma$ the gyromagnetic ratio, $\mathbf{h}_{\mathrm{eff},\nu}$ is the effective field including exchange field, dipolar field, and external field, $\alpha$ is the Gilbert damping and $J_\nu$ characterizes the strength of spin-orbit torques (SOTs) generated by the spin current, depending on the current flowing in the heavy metal layer, the spin Hall angle of the HM and the properties of the interface. Note that the the dissipation of magnon spin current caused by its interaction with the environment is phenomenologically covered by the Gilbert damping, while identifying its microscopic mechanism including spin-orbit interaction, spin pumping and two-magnon scattering [3] is not the focus of our current work.

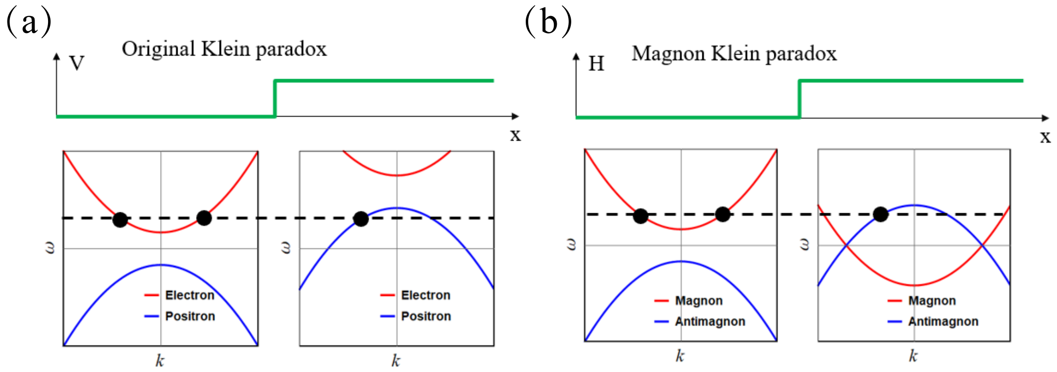


FIG. 1: Comparison between the original and magnon Klein paradox. The top panel (green line) sketches the “potential” distribution while the bottom panel sketches the dispersion relation of particles (red lines) and antiparticles (blue lines).

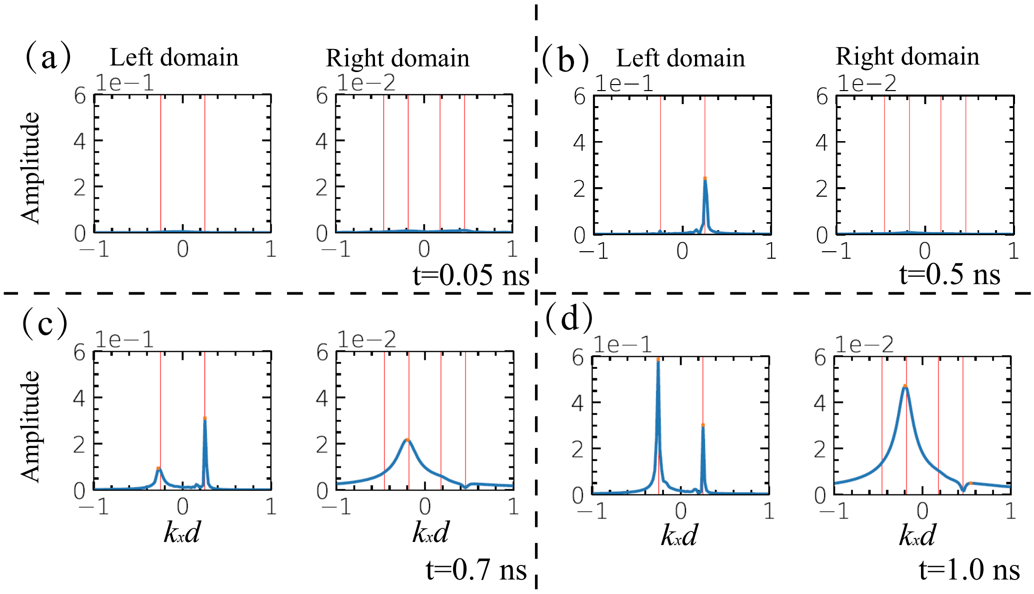


FIG. 2: Evolution of incident, reflected and transmitted magnons at $t$ = 0.05 ns (a), 0.5 ns (b), 0.7 ns (c) and 1.0 ns (d), respectively. The microwave source located on the left domain is turned on at $t = 0$ ns to excite magnons and then the magnons propagate toward the interface 800 nm away from the microwave source. All the other parameters are the same as Fig. 3(a) of the main text

The dimensions of the nanostrip on each domain are length $l = 2048$ nm, width $w = 64$ nm and thickness $d = 2$ nm. The SOT strength $J_L = 0$, and $J_R = J\hbar\theta_{SH}/(2M_s|e|d)$, where $J$ is current density, $\theta_{SH}$ is the spin-Hall angle of the heavy-metal layer, and $e$ is electron charge. Here we use the magnetic parameters of YIG/Pt, i.e., exchange coefficient $A = 3.1 \times 10^{-12}$ J/m, saturation magnetization $M_s = 1.92 \times 10^5$ A/m, spin-Hall angle $\theta_{SH} = 0.1$ [4], Gilbert damping $\alpha = 10^{-2}$. The inter-domain coupling $A_i$ is assumed to be a tunable coefficient and it is related to the coupling coefficient $J_c$ in the theory as $J_c = -2A_i/d$. The mesh size is $2 \times 2 \times 2$ nm$^3$. Absorptive boundary conditions are taken on the left domain to eliminate the influence of boundary reflection of magnons. The *Mumax*$^3$ [5] package is employed to numerically solve the LLG equation (1).

## CORRELATIONS OF INCIDENT, REFLECTED, AND TRANSMITTED MAGNON SPIN CURRENT

In the main text, we consider a classical model in which the antimagnons in the right domain can only be excited by an incoming magnon current from the left domain dynamically stabilized by SOTs. Without an incoming spin current from the left magnet, the right domain stays in the dynamically stabilized state, where the magnetization is pointing against the external field. Continuous emission of antimagnons would be present in a quantum mechanical treatment of the problem since there is no true ground state of the system. This can be interpreted as an analogue of Hawking radiation. Since we are considering a classical theory in this Letter, spontaneous emission of antimagnons is not captured by our classical model.

To verify the temporal correlation of antimagnon excitation and injected magnons, we plot the evolution of incident, reflected and transmitted magnon spin current in Fig. 2. Right after the microwave source located in the left domain is turned on, the excitations of both magnons and antimagnons are nearly zero [Fig. 2(a)], where the tiny excitations are mainly resulting from the fluctuation of spins in the ground state. Around 0.5 ns, the magnons on the left domain are significantly injected and propagate toward the interface [Fig. 2(b)]. Around 0.7 ns, the magnons reach the interface of left and right domains and inject the antimagnon current in the right domain [Fig. 2(c)]. Meanwhile, the reflected spin current appears and is amplified. As more antimagnons are excited, the reflection also becomes stronger [Fig. 2(d)]. This indeed verifies the temporal correlation between incident, reflected and transmitted magnon spin current.

* Electronic address: j.s.harms@uu.nl
† Electronic address: huaiyangyuan@gmail.com
[1] O. Klein, Z. Phys. **53**, 157 (1929).

[2] R. Brito, V. Cardoso, and P. Pani, arXiv:1501.06570v8.
[3] H. Y. Yuan, Y. Cao, A. Kamra, R. A. Duine, and P. Yan, arXiv:2111.14241.
[4] H. L. Wang, C. H. Du, Y. Pu, R. Adur, P. C. Hammel, and F. Y. Yang, Phys. Rev. Lett. **112**, 197201 (2014).
[5] A. Vansteenkiste, J. Leliaert, M. Dvornik, M. Helsen, F. Garcia-Sanchez, and F. B. V. Waeyenberge, AIP Adv. **4**, 107133 (2014).
